# Supplementary material for: Video-kMaX: A Simple Unified Approach for Online and Near-Online Video Panoptic Segmentation
Source: arXiv:2304.04694 source file (2023-04-10)
Supplement: Supplementary file 2 [file ablation_for_near_lamb_on_kitti_supple.tex]

% \begin{table}[t]
% \centering
% \small
% \tablestyle{3pt}{1.1}
\resizebox{0.92\linewidth}{!}{
\begin{tabular}{l|ccc|cc|c}
               & \multicolumn{3}{c|}{association features}  &  &  & \\
method         & video-stitching    & appearance      & location        & SQ      & AQ      & STQ       \\
\hline

        & \checkmark    &    &             & 74.2  &  72.3 &  73.3        \\
        &     & \checkmark  &                & 74.2    &   71.4   &     72.8 \\
        &     &      & \checkmark      &    74.2  &  72.3    & 73.2      \\
\modelname        &     & \checkmark & \checkmark      &  74.2     &  73.8    & 74.0      \\
(near-online)        & \checkmark    & \checkmark &      &    74.2  &    72.1  &   73.2  \\
        &  \checkmark   &  & \checkmark  & 74.2     &   73.6   & 73.9     \\
        &  \baseline{\checkmark}    &  \baseline{\checkmark} & \baseline{\checkmark}      & \baseline{74.2}     &  \baseline{74.2}    & \baseline{74.2}      \\
\end{tabular}}
% \vspace{-.8em}
% \caption{..}
% \label{tab:abla_near_lamb_kitti}
% \vspace{-2mm}
% \end{table}
