# Supplementary material for: Video-kMaX: A Simple Unified Approach for Online and Near-Online Video Panoptic Segmentation
Source: arXiv:2304.04694 source file (2023-04-10)
Supplement: Supplementary file 3 [file ablation_for_online_lamb_on_kitti_supple.tex]

% \begin{table}[t]
% \centering
% \small
% \tablestyle{3pt}{1.1}
\resizebox{0.92\linewidth}{!}{
\begin{tabular}{l|c|cc|cc|c}
                &   & \multicolumn{2}{c|}{association features} & & & \\
method & backbone  & appearance      & location        & SQ      & AQ      & STQ       \\
\hline
\multirow{8}{*}{$k$Max-DeepLab}
    & \multirow{4}{*}{ResNet50}   &     &                 &  75.0    & 10.0      & 27.3       \\
    &    & \checkmark    &                 &  75.0    & 33.8      &   50.4    \\
    &    &               & \checkmark       &   75.0   &   \textbf{72.0}   &   \textbf{73.5}   \\
\modelname    &    & \checkmark    & \checkmark       &   75.0   &   66.4   &   70.6   \\
    \cline{2-7}\cline{2-7}
(online)    &  \multirow{4}{*}{ConvNeXt-L}    &     &                 &  77.2  & 10.4      & 28.3      \\
    &    & \checkmark    &                 &  77.2    & 61.6      &   69.0    \\
    &    &               & \checkmark       &   77.2   &   74.0   &   75.6   \\
    &    & \baseline{\checkmark}    & \baseline{\checkmark}       &   \baseline{77.2}   &   \baseline{\textbf{75.7}}   &   \baseline{\textbf{76.5}}   \\
\end{tabular}}
% \vspace{-.8em}
% \caption{..}
% \label{tab:abla_online_lamb_kitti}
% \vspace{-2mm}
% \end{table}
